# Supplementary material for: QuasiSim: Parameterized Quasi-Physical Simulators for Dexterous Manipulations Transfer
Source: arXiv:2404.07988 source file (2024-07-21)
Supplement: Supplementary file 1 [file supp.tex]

% \tao{For both residual physics and residual force, people in this space are interested in their magnitude relative to the ``backbone'' physics and force. Ideally, the analytical model explains the majority of the physics and the residual one serves a minor role. I think it would be good if you happen to have such data and report whether this is indeed the case.}
